# Supplementary material for: CaFA: Global Weather Forecasting with Factorized Attention on Sphere
Source: arXiv:2405.07395 source file (2024-05-12)

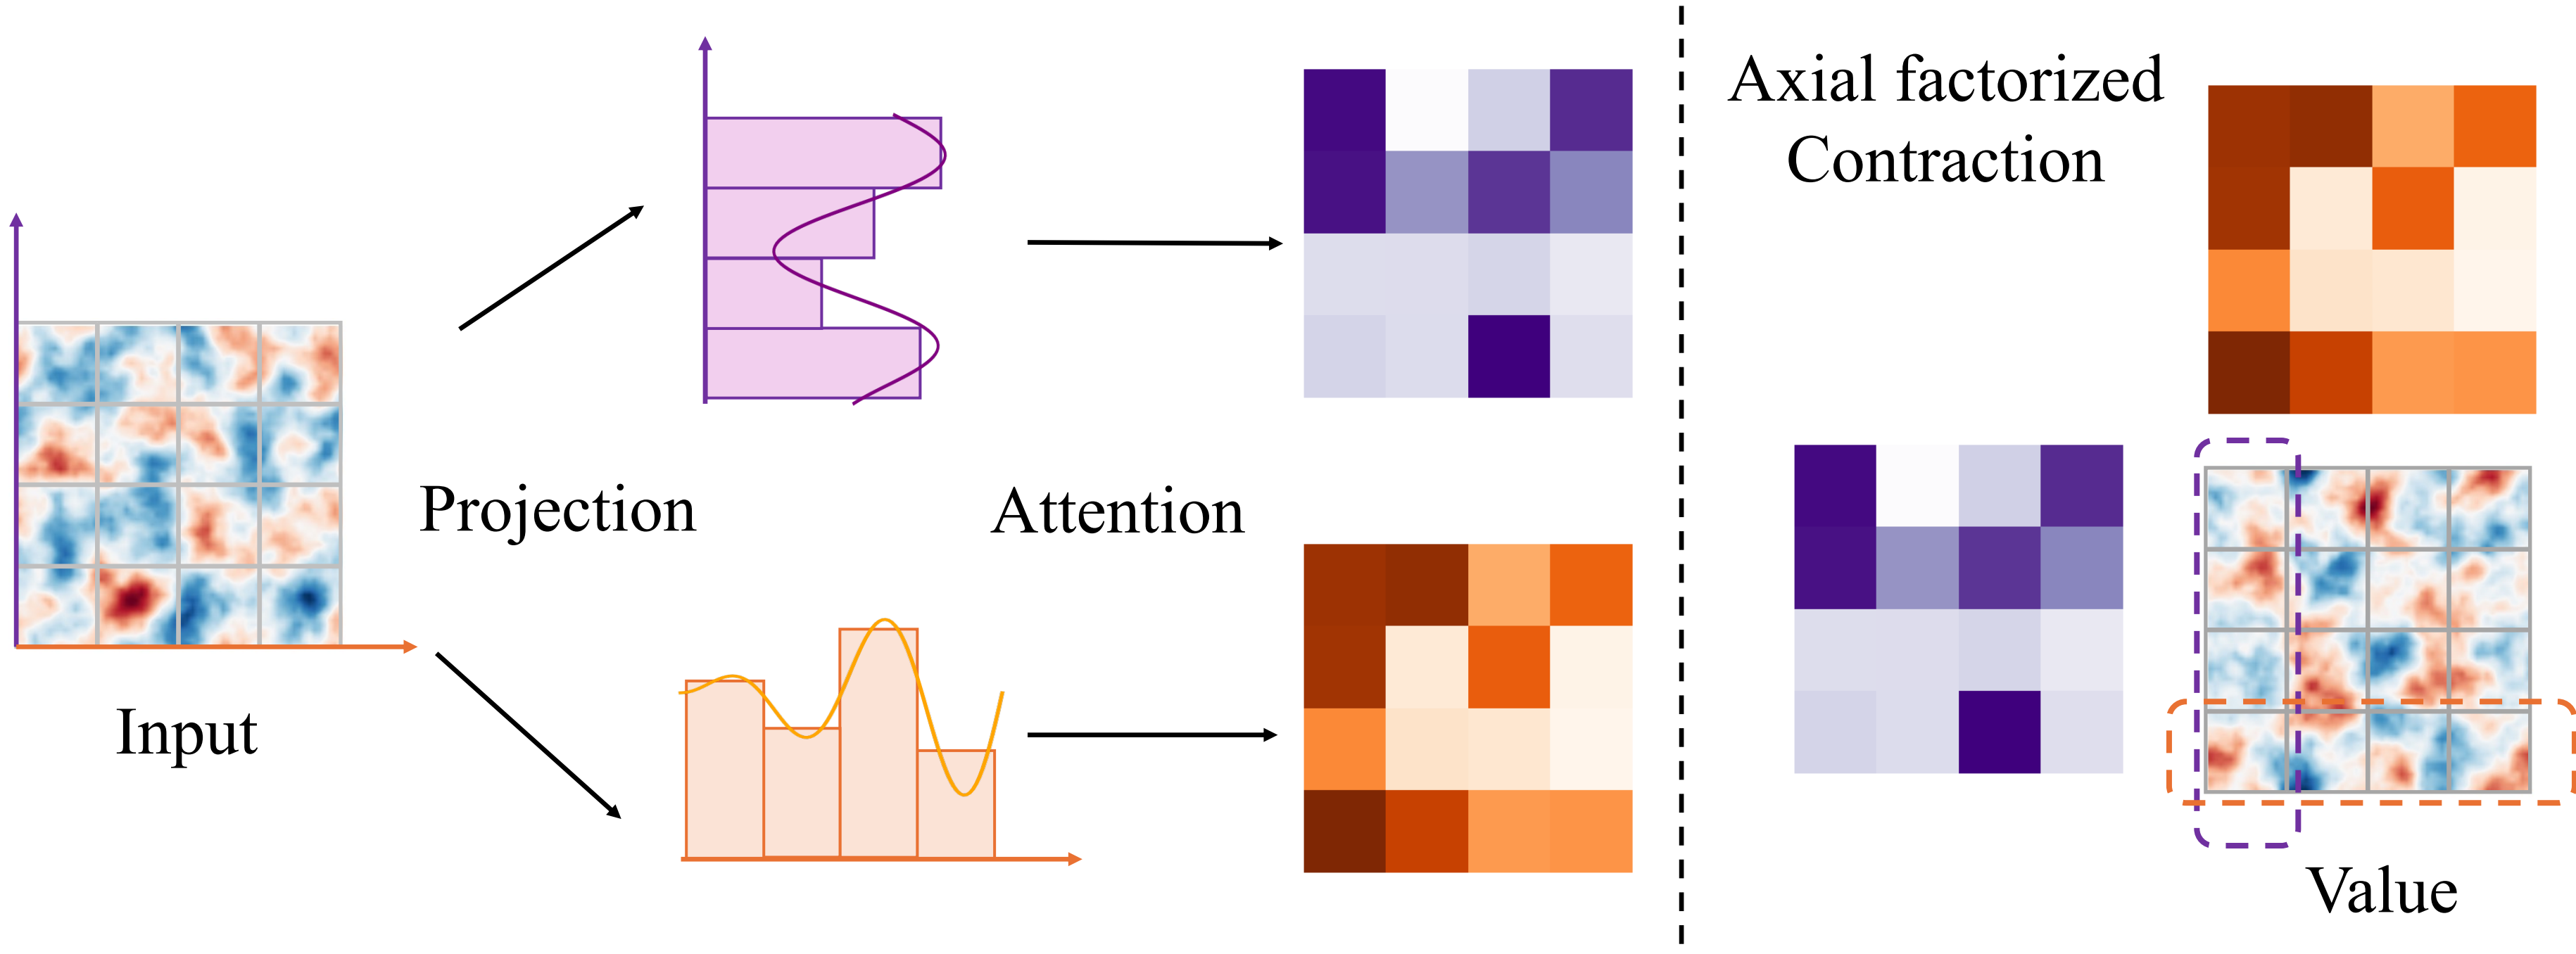

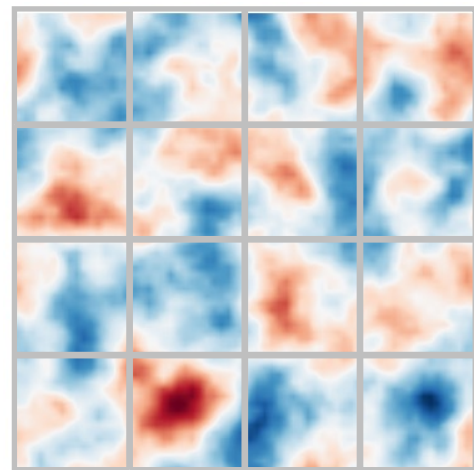

Spatial structure  
flattening

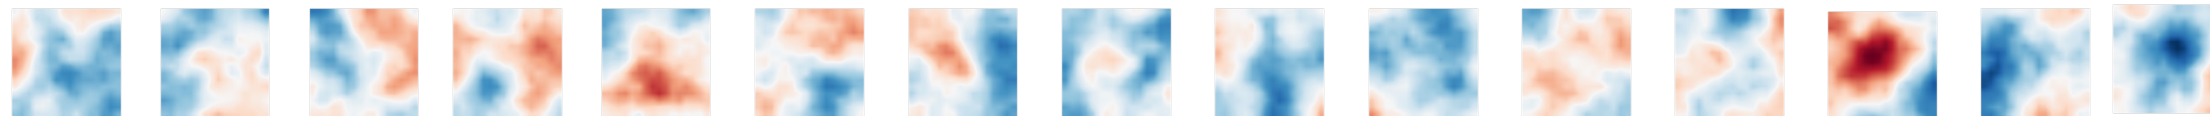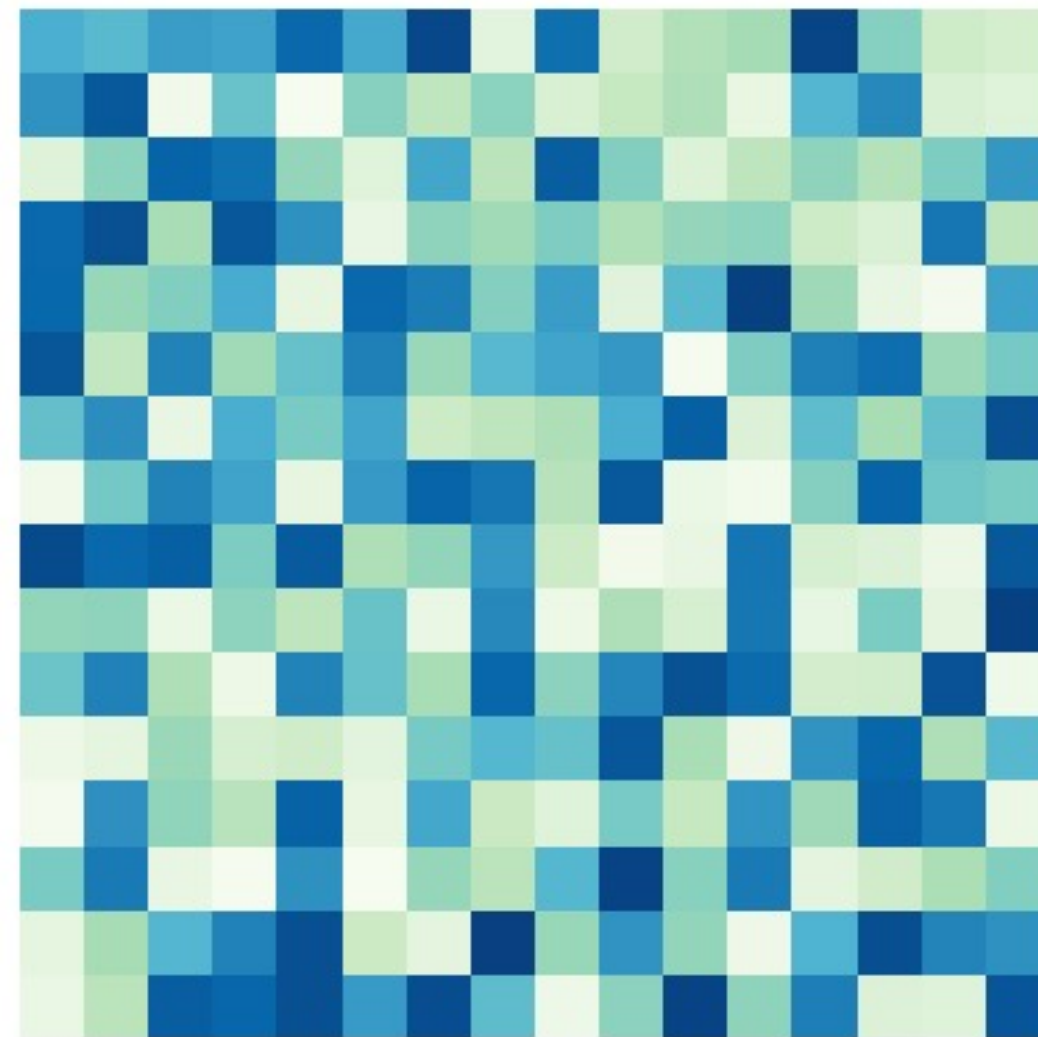

Full attention

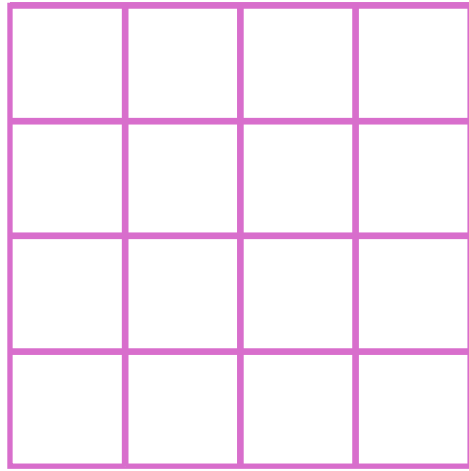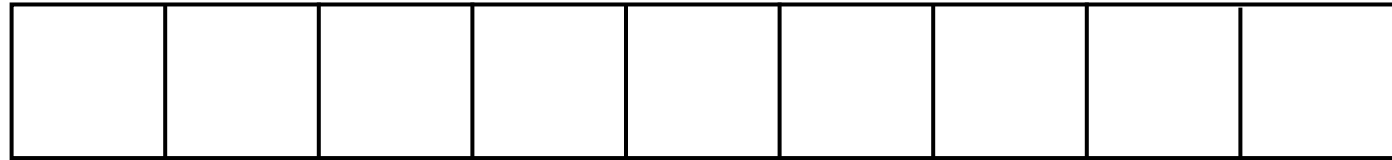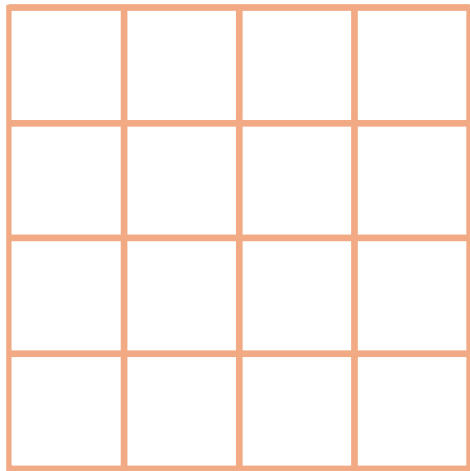

Supplement: Supplementary file 1 [file Diagram_factorized_attention.pdf]
